# Supplementary material for: Face Forensics in the Wild
Source: arXiv:2103.16076 source file (2021-03-30)
Supplement: Supplementary file 1 [file 06136-supp.pdf]

# *Supplemental Material*: Face Forensics in the Wild


Tianfei Zhou[1] , Wenguan Wang[1*] , Zhiyuan Liang[2] , Jianbing Shen[3,2]

[1]ETH Zurich [2]Beijing Institute of Technology [3]Inception Institute of Artificial Intelligence

https://github.com/tfzhou/FFIW


This document provides additional materials to supplement our main manuscript. We first present more details about Q-Net in §1, and then provide additional quantitative results on $FFIW_{10K}$ `val` in §2. Finally, we offer extra statistics and visual examples of $FFIW_{10K}$ in §3.

## 1. More Details on Q-Net

**Detailed Network Architecture.** We employ VGG16 [11] as the backbone network of Q-Net. Let $\boldsymbol{q} \in \mathbb{R}^{512}$ denote the backbone feature. Two small multi-layer perceptrons are further added for score regression and domain adversarial learning, respectively. The score regression head has the following architecture: $\boldsymbol{q}\rightarrow$FC(1024)$\rightarrow$FC(1024)$\rightarrow$FC(2), and the domain adversarial head is implemented as: $\boldsymbol{q}\rightarrow$FC(1024)$\rightarrow$FC(1024)$\rightarrow$FC(3). Here, FC means a fully-connected layer.

**Training Details.** We train Q-Net using the SGD optimizer with a min-batch size of 128, learning rate of 1e-4 and momentum of 0.9. All the training images are resized to 224×224. During training, the domain-regularization parameter $\alpha$ is initialized as 0 and gradually increased to 1 following the schedule [5]:

$$\alpha = \frac{2}{1+\exp(-10t)} - 1, \text{where } t = n/N. \tag{1}$$

Here, $n$ and $N$ indicate the number of current epoch and total epoch, respectively. This strategy enables the domain classifier to be more robust to noisy signal at the early stages of the training procedure.

**User Study.** In order to evaluate the performance of Q-Net, we carry out a user study to examine the consistency between model predictions and human assessments. Specifically, we randomly select 2,000 pairs of swapped faces. Each pair is then presented to three humans to determine which face is of better quality. We note that for some pairs, both faces may be in a similar quality level, under which condition it will be difficult for humans or Q-Net to determine the correct ranking. To this end, we discard such pairs and only keep the pairs that all three observers have consistent opinions. This finally leads to a total of 1,357 pairs. For each remaining pair, its Q-Net ranking is regarded correct if it is consistent with the human ranking. The overall accuracy of Q-Net ranking on the 1,357 pairs is ***85.63%***, showing a strong consistency with human assessment.

In addition, to guarantee the quality of tampered faces in $FFIW_{10K}$, we need to determine a suitable quality threshold so that tampered faces with quality scores below the threshold can be regarded as low quality and thus can be simply discarded. Another user study has been conducted for this. In particular, we collect 4,000 samples whose quality scores fall into ranges $[0.4, 0.5)$, $[0.5, 0.6)$, $[0.6, 0.7)$, or $[0.7, 0.8)$, 1,000 samples for each range. For each sample, we present it to three human observers for rating it at five levels (*i.e.*, clearly fake, fake, borderline, real, clearly real). Then, a sample is considered as high-quality if a majority of its three rates are 'real' or 'clearly real'. The results are summarized in Table 1. As seen, ***89.5%*** samples with scores in $[0.6, 0.7)$ are regarded as high-quality. Although the ratio is slightly higher for the range $[0.7, 0.8)$, we find that more high-fidelity faces will be discarded if only considering the samples with scores above 0.7. Therefore, we select 0.6 as the final threshold.

| score ranges | $[0.4, 0.5)$ | $[0.5, 0.6)$ | $[0.6, 0.7)$ | $[0.7, 0.8)$ |
|---|---|---|---|---|
| number of test sample | 1,000 | 1,000 | 1,000 | 1,000 |
| ratio of high-quality samples | 43.9% | 67.6% | 89.5% | 91.3% |

Table 1: Results of the user study to determine the quality threshold.

**Qualitative Results.** Fig. 1 shows some tampered faces along with their quality scores predicted by Q-Net. We see that Q-Net can make accurate predictions that well align with human perception.

## 2. More Quantitative Result

We show benchmarking results of all methods on the `val` set of $FFIW_{10K}$ in Table 2. We see that the results well align with those in $FFIW_{10K}$ `test`, as reported in Table 2 of the main manuscript. The proposed approach achieves the best performance across all metrics, using only video-level labels for training.


*Corresponding author: *Wenguan Wang*.

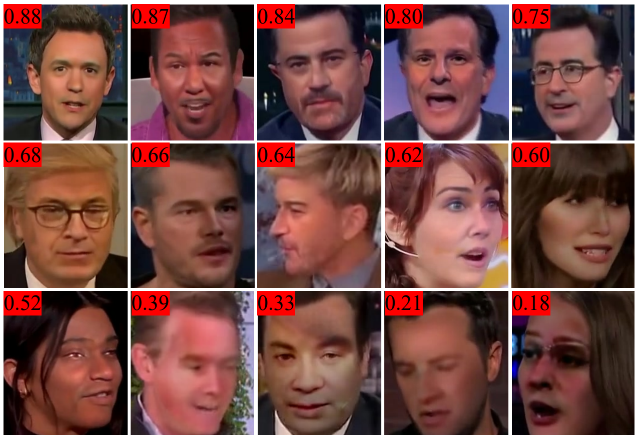


Figure 1: Visualizations of tampered faces along with corresponding quality scores predicted by Q-Net.

| Methods | classification ACC (%) | classification AUC (%) | localization mAP (%) |
|---|---|---|---|
| frame-based methods: using face-level labels as supervision | | | |
| Xception [10] | 55.3 | 57.0 | 18.6 |
| MesoNet [2] | 56.7 | 58.1 | 19.2 |
| PatchForensics [4] | 60.3 | 63.4 | 19.5 |
| FWA [7] | 60.9 | 63.7 | 19.6 |
| video-based methods: using face-level labels as supervision | | | |
| TSN [13] | 63.1 | 64.6 | 22.5 |
| C3D [12] | 65.5 | 66.3 | 24.7 |
| I3D [3] | 70.9 | 71.7 | 30.8 |
| video-based methods: using video-level labels as supervision | | | |
| S-MIL [6] | 60.8 | 62.3 | - |
| **Ours** | **71.3** | **73.5** | **31.1** |

Table 2: **Quantitative results on `val` set of *FFIW*$_{10K}$.** The best scores are highlighted in **bold**.

## 3. *FFIW*$_{10K}$ Dataset

**More Statistics.** In Table 3, we summarize the number of forged videos generated by each of the three face swapping methods (*i.e.*, FSGAN [8], DeepFaceLab [9], FaceSwap [1]) in *FFIW*$_{10K}$. We see that a majority of videos are generated by FSGAN [8] because the algorithm is of high efficiency and thus allows for large-scale video manipulation. DeepFaceLab[9] generally creates videos with higher qualities than FSGAN, however, the approach requires expensive training procedure for each manipulation, limiting its practical application. FaceSwap [1] is a non-learning method which is fast but with poor generation performance. We emphasize that all the videos in *FFIW*$_{10K}$ are selected by Q-Net to guarantee the high quality.

For completeness, we offer the statistics regarding gender and video resolution in Fig. 2. The distributions well align with real-world data distributions.

| Methods | FSGAN [8] | DeepFaceLab [9] | FaceSwap [1] |
|---|---|---|---|
| # fake videos | 5,800 | 2,200 | 2,000 |

Table 3: **Statistics of the number of videos** manipulated by each of the three face swapping approaches.

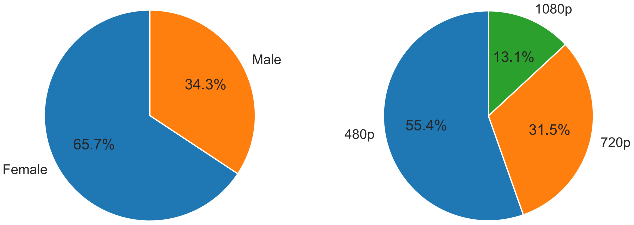


Figure 2: Left: Gender distribution over all manipulated videos. Right: Video resolution distribution of pristine video clips.

**More Visual Examples.** In Fig. 3 and Fig. 4, we present additional visual examples in the proposed dataset, *i.e.*, *FFIW*$_{10K}$. The synthetic faces are highlighted by red boxes, and zoomed in for clear presentation. We see that *FFIW*$_{10K}$ provides high-fidelity tampered faces in various challenging cases (*e.g.*, multiple faces, cluttered background, small scale, profile faces). This makes *FFIW*$_{10K}$ well suitable for training and evaluating face forgery detection methods, especially in multi-person scenarios.

## References

[1] Faceswap. https://github.com/MarekKowalski/FaceSwap/. accessed November 10, 2020. 2
[2] Darius Afchar, Vincent Nozick, Junichi Yamagishi, and Isao Echizen. Mesonet: a compact facial video forgery detection network. In *WIFS*, 2018. 2
[3] João Carreira, Andrew Zisserman, and Quo Vadis. Action recognition? a new model and the kinetics dataset. In *CVPR*, 2018. 2
[4] Lucy Chai, David Bau, Ser-Nam Lim, and Phillip Isola. What makes fake images detectable? understanding properties that generalize. In *ECCV*, 2020. 2
[5] Yaroslav Ganin, Evgeniya Ustinova, Hana Ajakan, Pascal Germain, Hugo Larochelle, François Laviolette, Mario Marchand, and Victor Lempitsky. Domain-adversarial training of neural networks. *JMLR*, 17(1):2096–2030, 2016. 1
[6] Xiaodan Li, Yining Lang, Yuefeng Chen, Xiaofeng Mao, Yuan He, Shuhui Wang, Hui Xue, and Quan Lu. Sharp multiple instance learning for deepfake video detection. In *ACM MM*, 2020. 2
[7] Yuezun Li and Siwei Lyu. Exposing deepfake videos by detecting face warping artifacts. *arXiv preprint arXiv:1811.00656*, 2018. 2
[8] Yuval Nirkin, Yosi Keller, and Tal Hassner. Fsgan: Subject agnostic face swapping and reenactment. In *ICCV*, 2019. 2
[9] Ivan Petrov, Daiheng Gao, Nikolay Chervoniy, Kunlin Liu, Sugasa Marangonda, Chris Umé, Jian Jiang, Luis RP, Sheng Zhang, Pingyu Wu, et al. Deepfacelab: A simple, flexi-

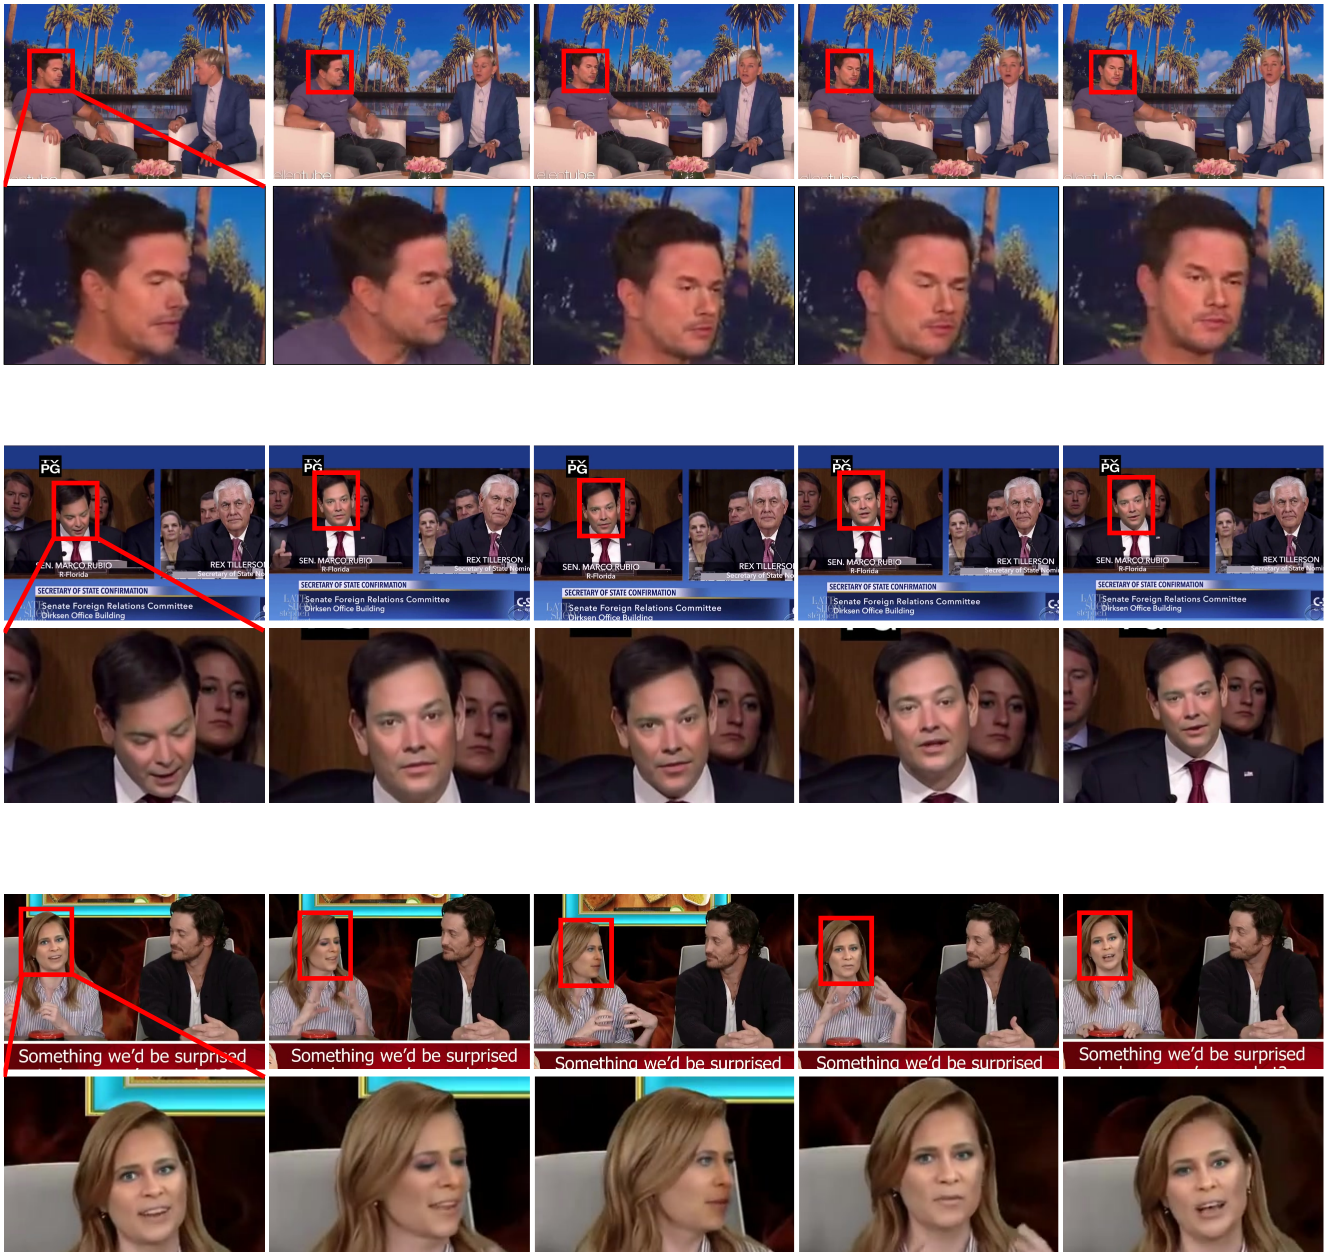


Figure 3: More visual examples in $\textit{FFIW}_{10K}$. The forged faces are highlighted by red boxes, and zoomed in for clear presentation.

ble and extensible face swapping framework. *arXiv preprint arXiv:2005.05535*, 2020. 2

[10] Andreas Rossler, Davide Cozzolino, Luisa Verdoliva, Christian Riess, Justus Thies, and Matthias Nießner. Faceforensics++: Learning to detect manipulated facial images. In *ICCV*, 2019. 2

[11] Karen Simonyan and Andrew Zisserman. Very deep convolutional networks for large-scale image recognition. *arXiv preprint arXiv:1409.1556*, 2014. 1

[12] Du Tran, Lubomir Bourdev, Rob Fergus, Lorenzo Torresani, and Manohar Paluri. Learning spatiotemporal features with 3d convolutional networks. In *ICCV*, 2015. 2

[13] Limin Wang, Yuanjun Xiong, Zhe Wang, Yu Qiao, Dahua Lin, Xiaoou Tang, and Luc Van Gool. Temporal segment networks: Towards good practices for deep action recognition. In *ECCV*, 2016. 2

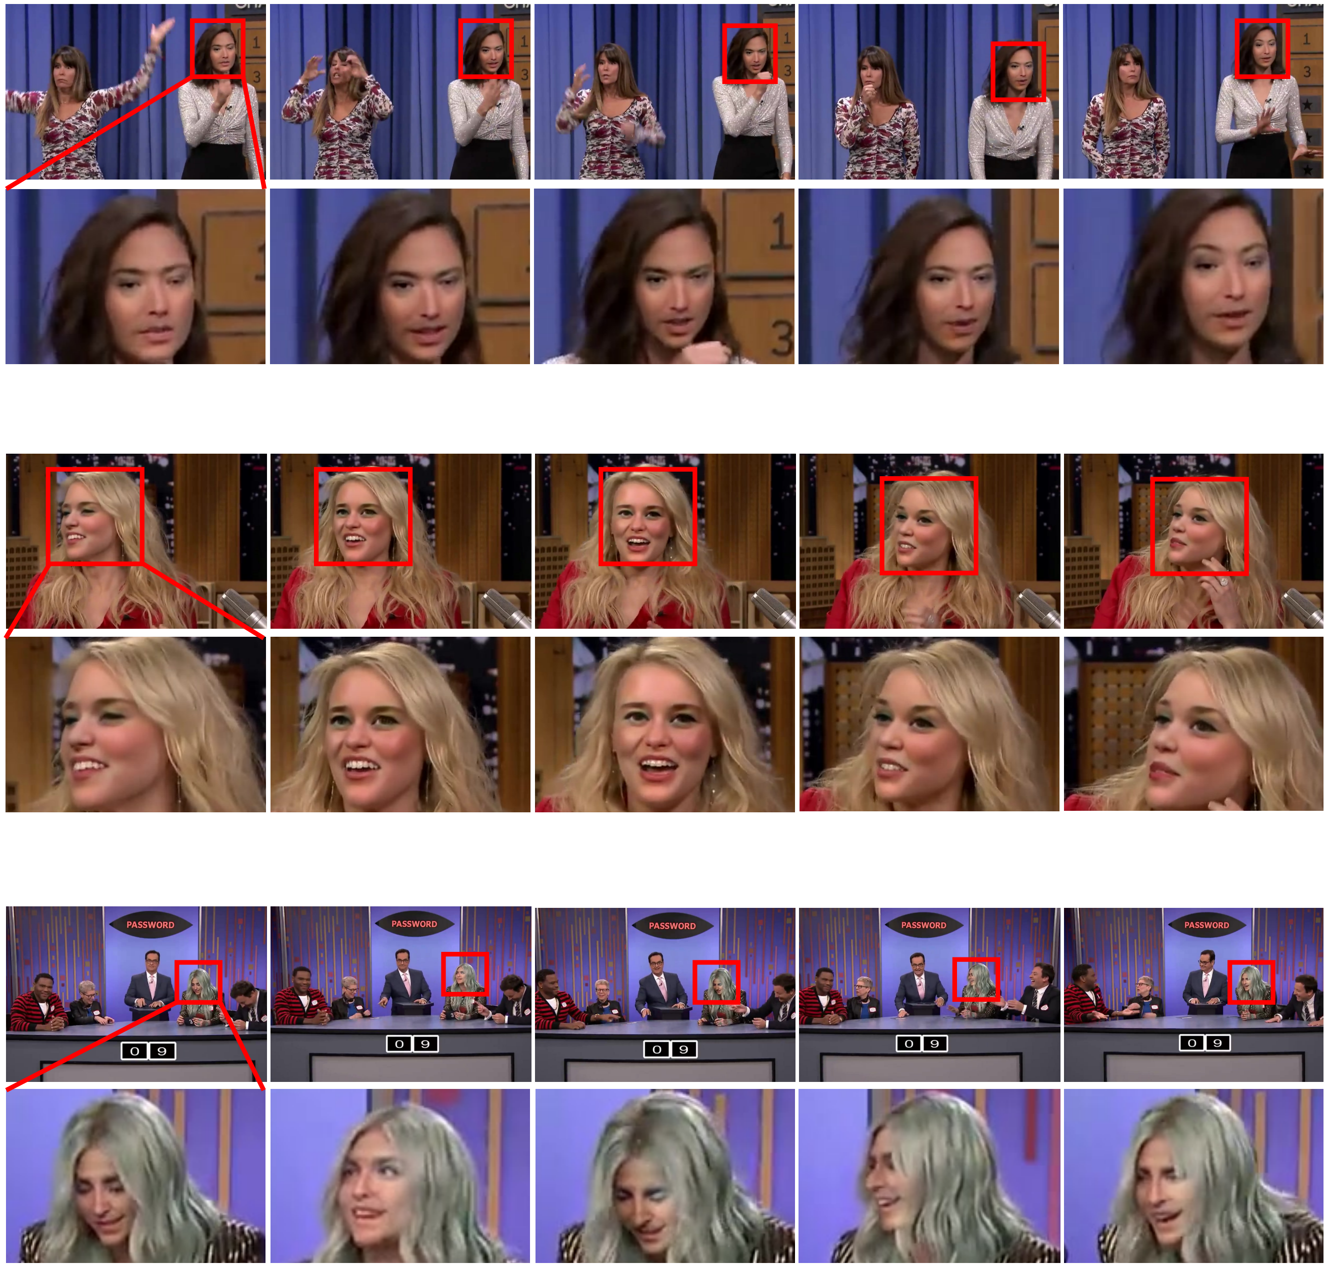


Figure 4: More visual examples in $FFIW_{10K}$. The forged faces are highlighted by red boxes, and zoomed in for clear presentation.
